# Supplementary material for: Tractable Lineages on Treelike Instances: Limits and Extensions
Source: arXiv:1604.02761 source file (2023-04-12)
Supplement: Supplementary file 1 [file appendix.tex]

\section{Differences with~\lowercase{\cite{amarilli2015provenance}}}
\label{apx:differences}
We point out some differences in definitions in comparison
with~\cite{amarilli2015provenance}.

\paragraph*{Tree decompositions} In~\cite{amarilli2015provenance} tree
decompositions are always binary trees, and are transformed into binary
tree encodings with a single fact per node. We can thus
use tree automata over ranked trees to process the encodings.
In the current article, tree
decompositions are defined through arbitrary (unranked) trees. This
is not a substantial difference: in particular, this does not change the
treewidth (given an unranked tree, it is always possible to duplicate a
node keeping the exact same bag of vertices, to form a binary tree structure).

\paragraph*{Treewidth of circuits}
This paper defines the \emph{treewidth} of a circuit (see
Definition~\ref{def:circuit} and remark afterward) as the treewidth of
the DAG that represents it. By contrast, the \emph{treewidth} of a circuit is
defined in~\cite{amarilli2015provenance} as that of a relational representation
of the circuit, where each gate has been rewritten using associativity to have
fan-in of at most two. The two notions of treewidth are different, but they are within
a factor of~$3$ of each other. Indeed, considering a circuit rewritten using
associativity, consider a tree decomposition of the circuit in the sense defined in this
paper. One can obtain a tree decomposition of the relational representation of
the circuit by adding, for each gate $g$ and each bag where it occurs, its incoming
nodes (of which there are at most two). This clearly gives a tree decomposition,
because the subtree of occurrences of~$g$ must be connected to that of its
incoming gates, so the occurrences of each gate in the rewritten decomposition
are still a connected subtree. Further, any fact in the relational
representation is now covered. The width of the rewritten decomposition is at
most three times that of the original decomposition.

\paragraph*{Domain semantics}
In this paper, we explicitly adopt the \emph{active domain semantics}, where the
domain of an instance consists exactly of the elements that occur in facts. By
contrast~\cite{amarilli2015provenance} (implicitly) adopts a semantics where the
domain of instances may be different from the active domain. Specifically, when
considering the possible subinstances $I' \subseteq I$ of an instance~$I$, the
semantics used there is that $\dom(I') = \dom(I)$ in all cases. This makes no
difference for queries in \ucq (where variables always occur in some atom), but
can make a difference for more general queries.

This difference is inessential, however. Indeed, we can ensure that
\cite{amarilli2015provenance} follows the active domain semantics, by the standard
technique of relativized quantifiers. Formally, whenever we quantify over a
variable, we add a disjunction stating that the variable occurs in some atom.
As~\cite{amarilli2015provenance} allows queries in MSO, we can perform this
transformation and remain in the same language.
